# Supplementary material for: N$_2$, NO and O$_2$ molecules in LiGaO$_2$ in both Ga and Li sites and their relation to the vacancies
Source: arXiv:2201.05516 source file (2022-01-14)
Supplement: Supplementary file 1 [file Supplementary_information.pdf]

**Supplementary information for**

# "$N_2$, NO and $O_2$ molecules in $LiGaO_2$ in both Ga and Li sites and their relation to the vacancies"

Klichchupong Dabsamut,[1, 2] Adisak Boonchun[1, a] and Walter Lambrecht[2, b]

[1]Department of Physics, Faculty of Science, Kasetsart University, Bangkok 10900 Thailand
[2]Department of Physics, Case Western Reserve University, 10900 Euclid Avenue, Cleveland, Ohio 44106-7079, USA

[a]E-mail: adisak.bo@ku.th
[b]E-mail: walter.lambrecht@case.edu

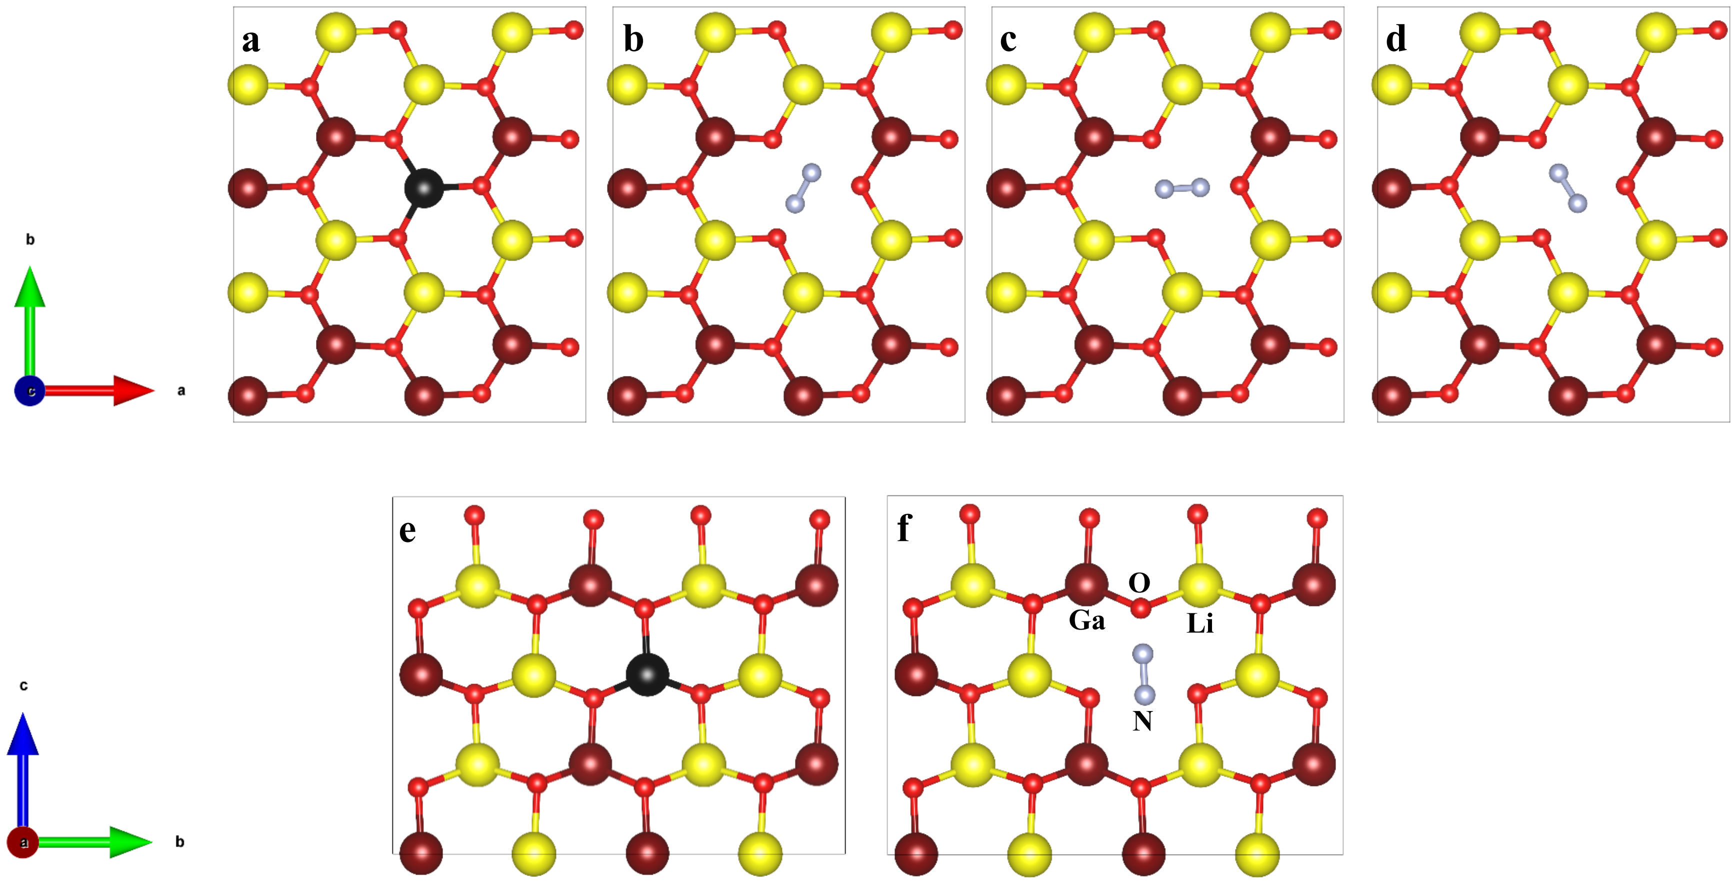


**Fig. S1.** The initial structures of planar configurations ( (a) original Ga site, (b) P1, (c) P2 and (d) P3 ) and vertical configuations ( (e) original Ga site and (f) V1 ) for $N_2$ and $O_2$ in Ga site. We note that we removed other layers of $LiGaO_2$ to make it easier to spot the molecules.

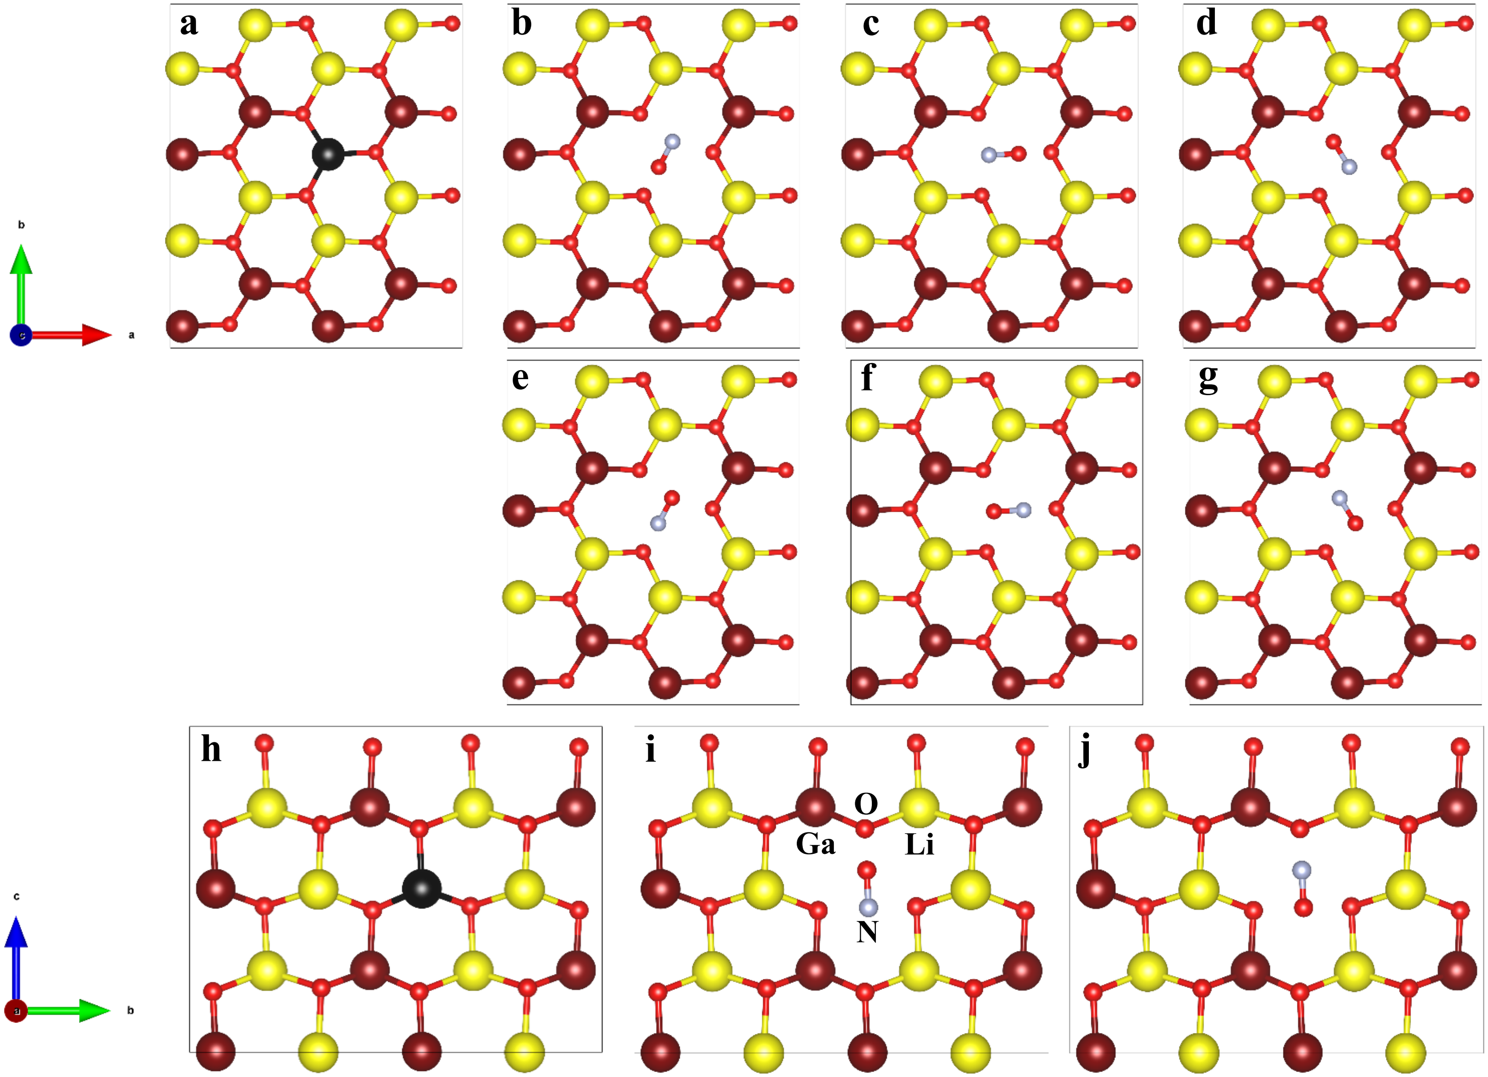


**Fig. S2.** The initial structures of planar configurations ( (a) original Ga site, (b) P1-a, (c) P2-a, (d) P3-a, (e) P1-b, (f) P2-b and (g) P3-b ) and vertical configuations ( (h) original Ga site, (i) V1-a and (j) V1-b for NO in Ga site. We note that we removed other layers of $LiGaO_2$ to make it easier to spot the molecules.

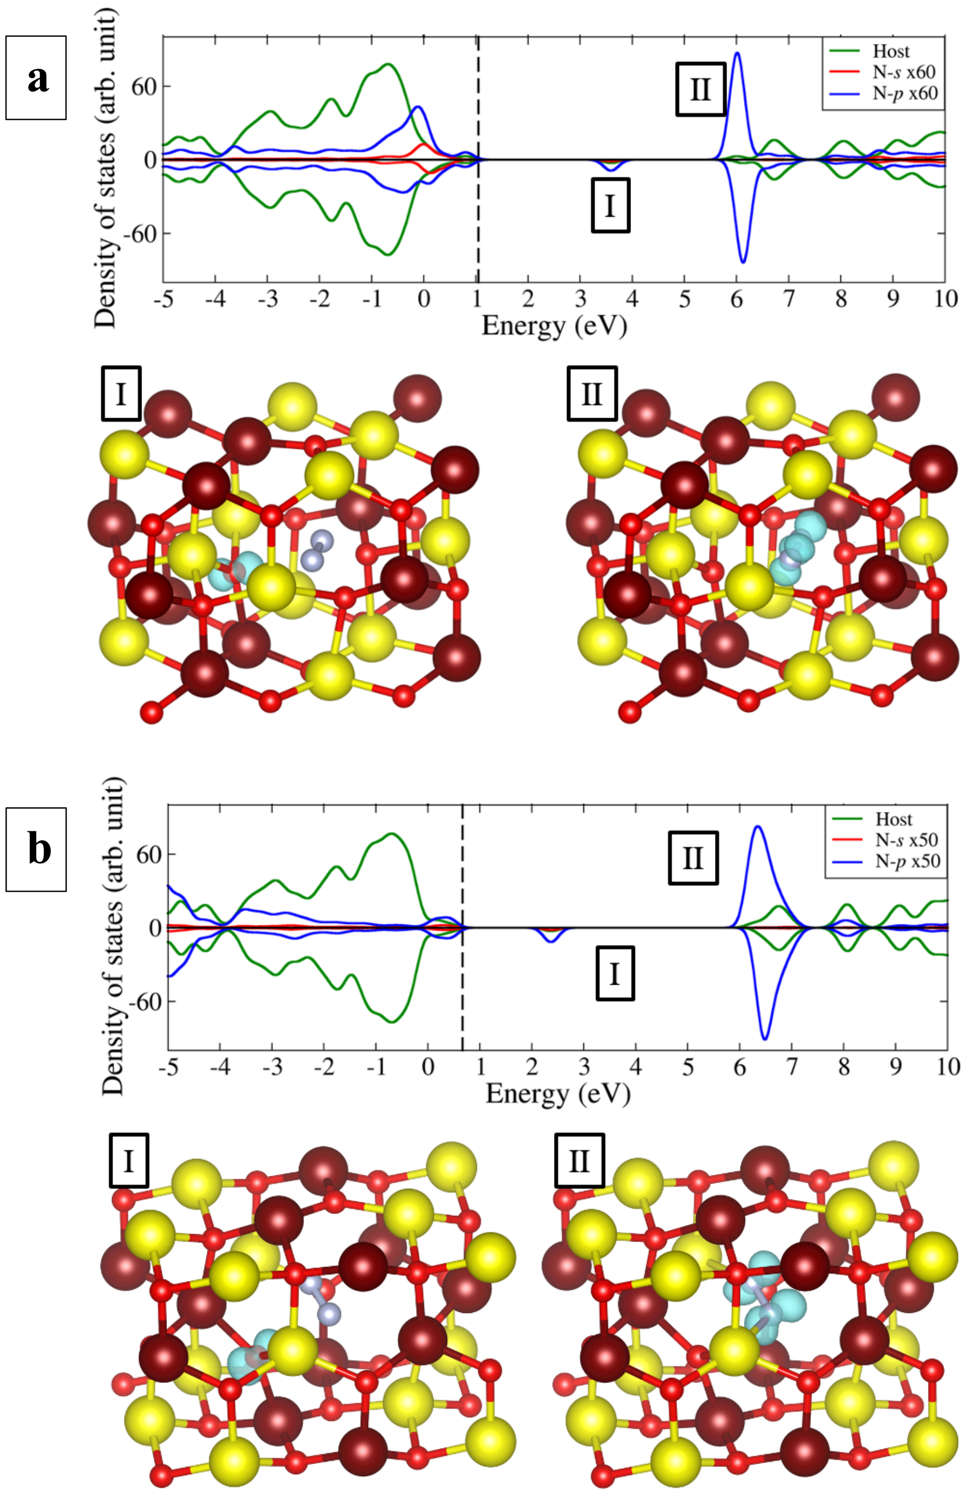


**Fig S3.** The partial density of state (PDOS) and the wave function localization of (a) $(N_2)_{Ga}$ and (b) $(N_2)_{Li}$, respectively, both in the neutral charge state. We note that the dashed line separates the occupied and unoccupied state.

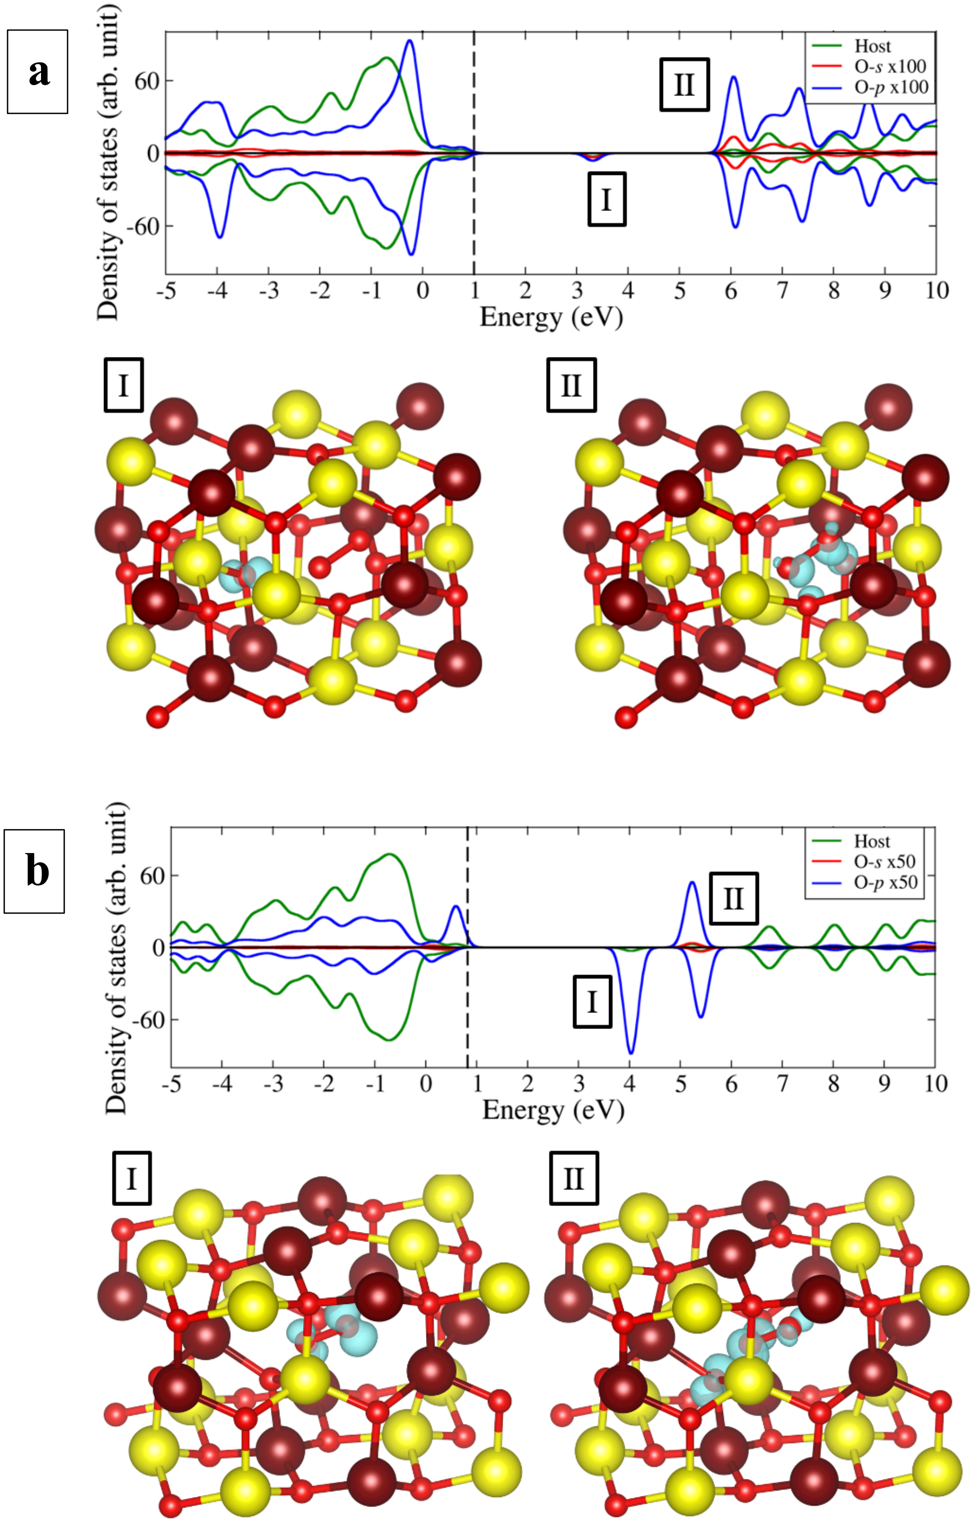


**Fig S4.** The partial density of state (PDOS) and the wave function localization of neutral (a) $(O_2)_{Ga}$ and (b) $(O_2)_{Li}$, respectively. We note that the dash line separates the occupied and unoccupied state.

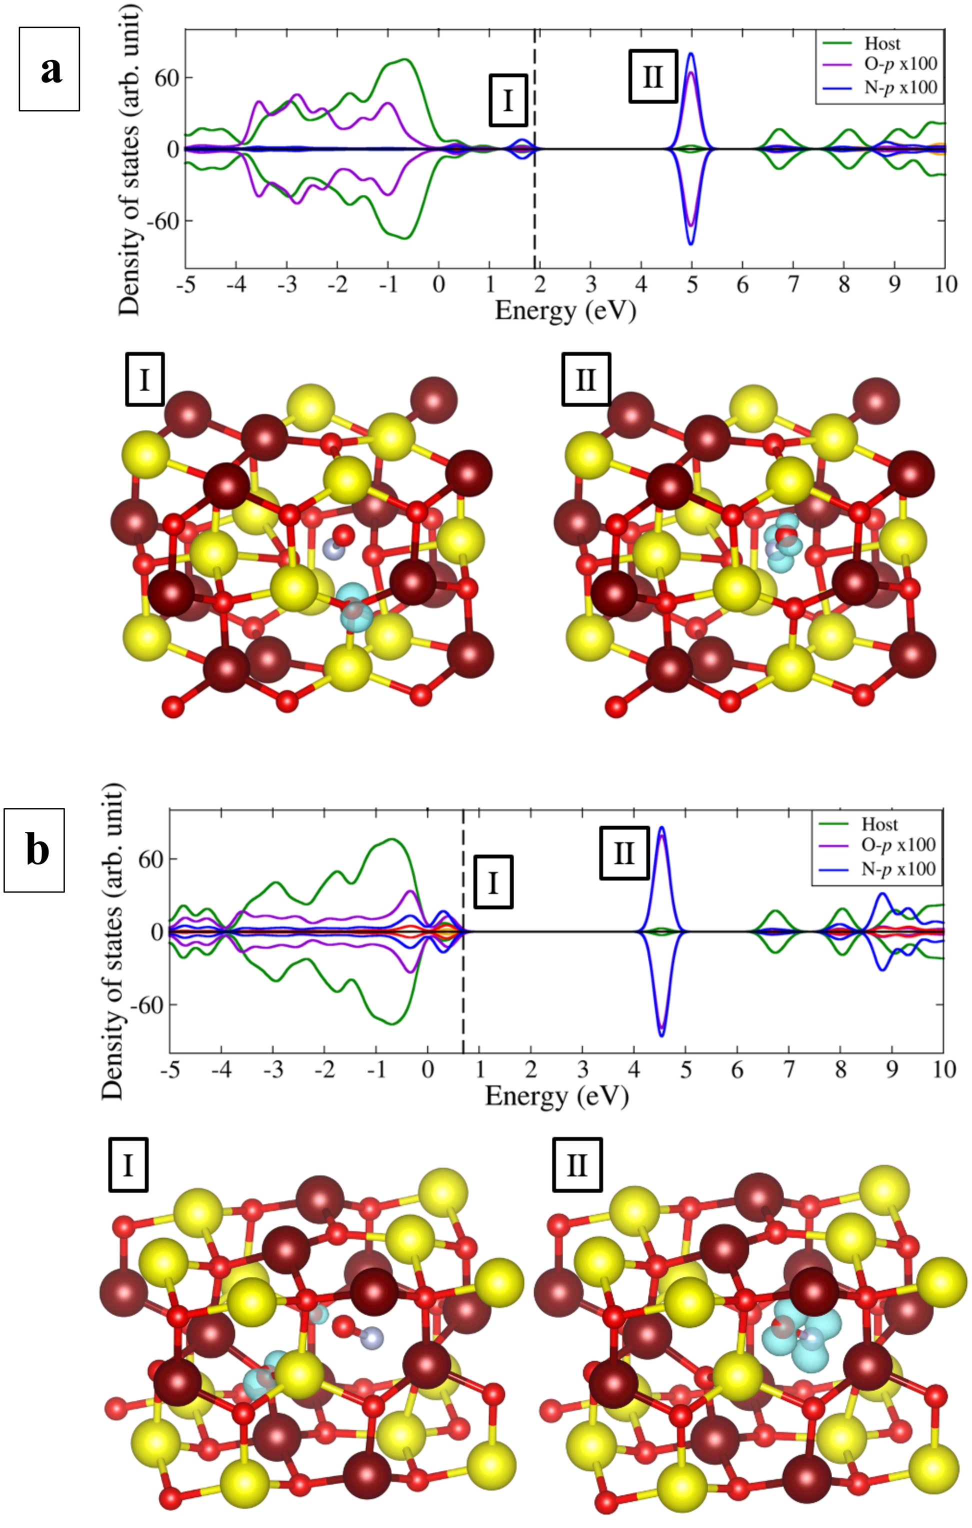


**Fig S5.** The partial density of state (PDOS) and the wave function localization of neutral (a) $(NO)_{Ga}$ and (b) $(NO)_{Li}$, respectively. We note that the dash line separates the occupied and unoccupied state.

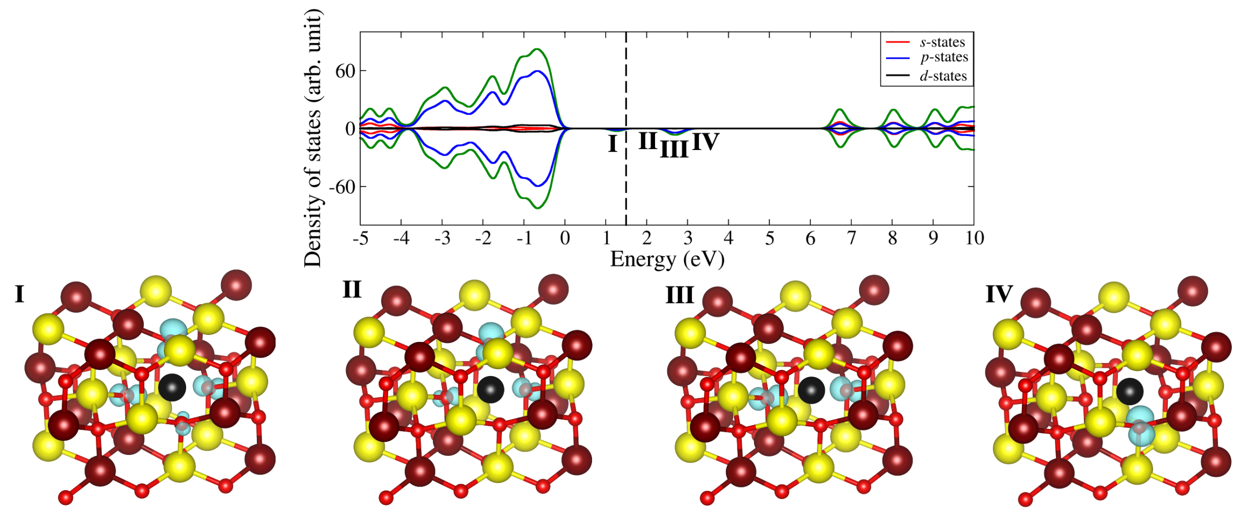


**Fig S6.** The partial density of state (PDOS) and the wave function localization of $V_{\mathrm{Ga}}$. We note that the dash line separates the occupied and unoccupied state.

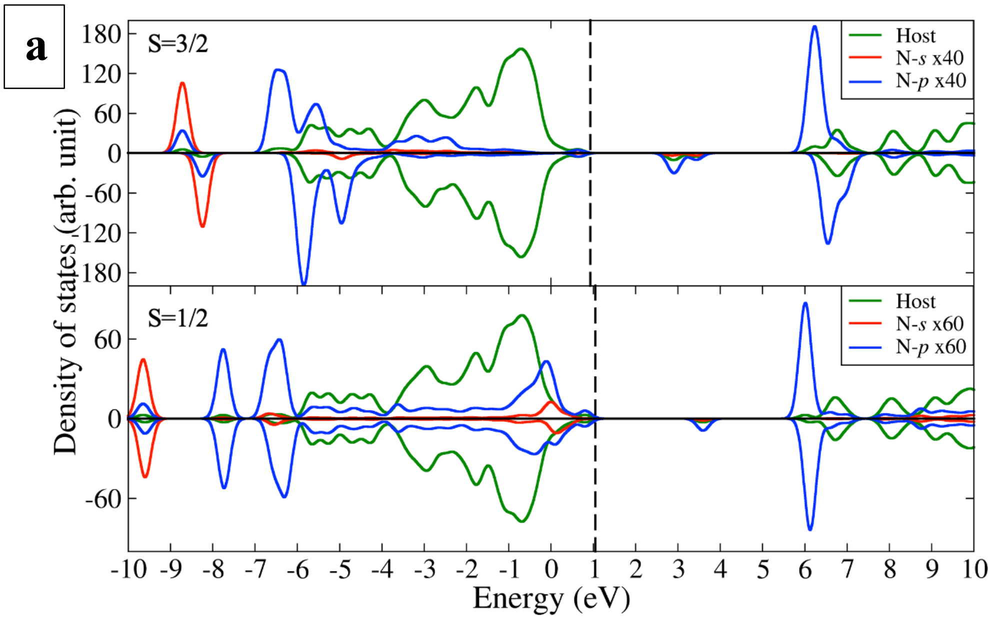


| S | Energy/128-atom-supercell (eV) |
|---|---|
| 3/2 | -898.25 |
| 1/2 | -899.78 |

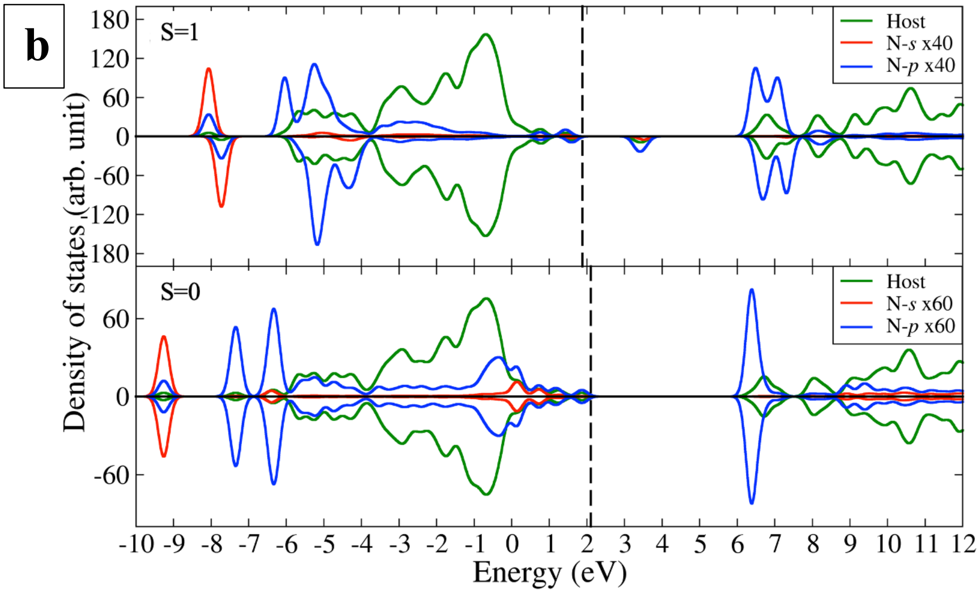


| S | Energy/128-atom-supercell (eV) |
|---|---|
| 1 | -895.82 |
| 0 | -896.87 |

**Fig S7.** The comparison of PDOS and energy/supercell in high and low spin states of $(N_2)_{Ga}$ with (a) neutral charge state and (b) -1 charge state, respectively.

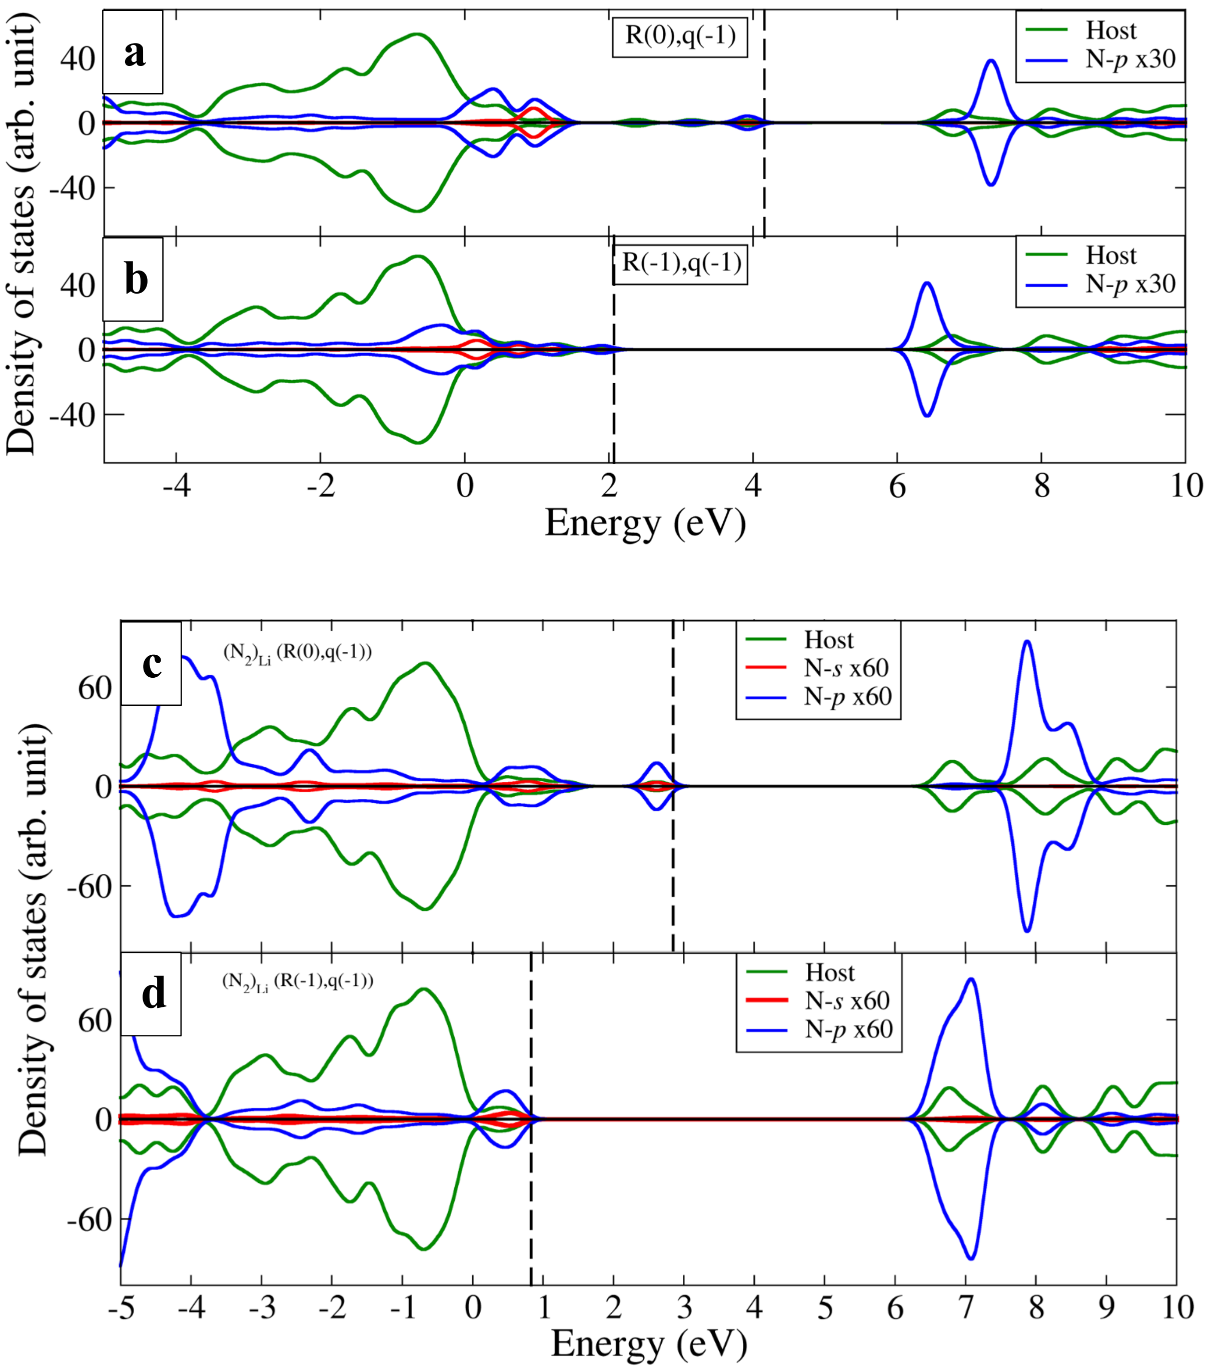


**Fig S8.** The PDOS of $(N_2)_{Ga}$ negative charge state with (a) frozen geometry of the neutral state and (b) relaxzation structure, and the PDOS of $(N_2)_{Li}$ negative charge state with (c) frozen geometry of the neutral state and (d) relaxzation structure.

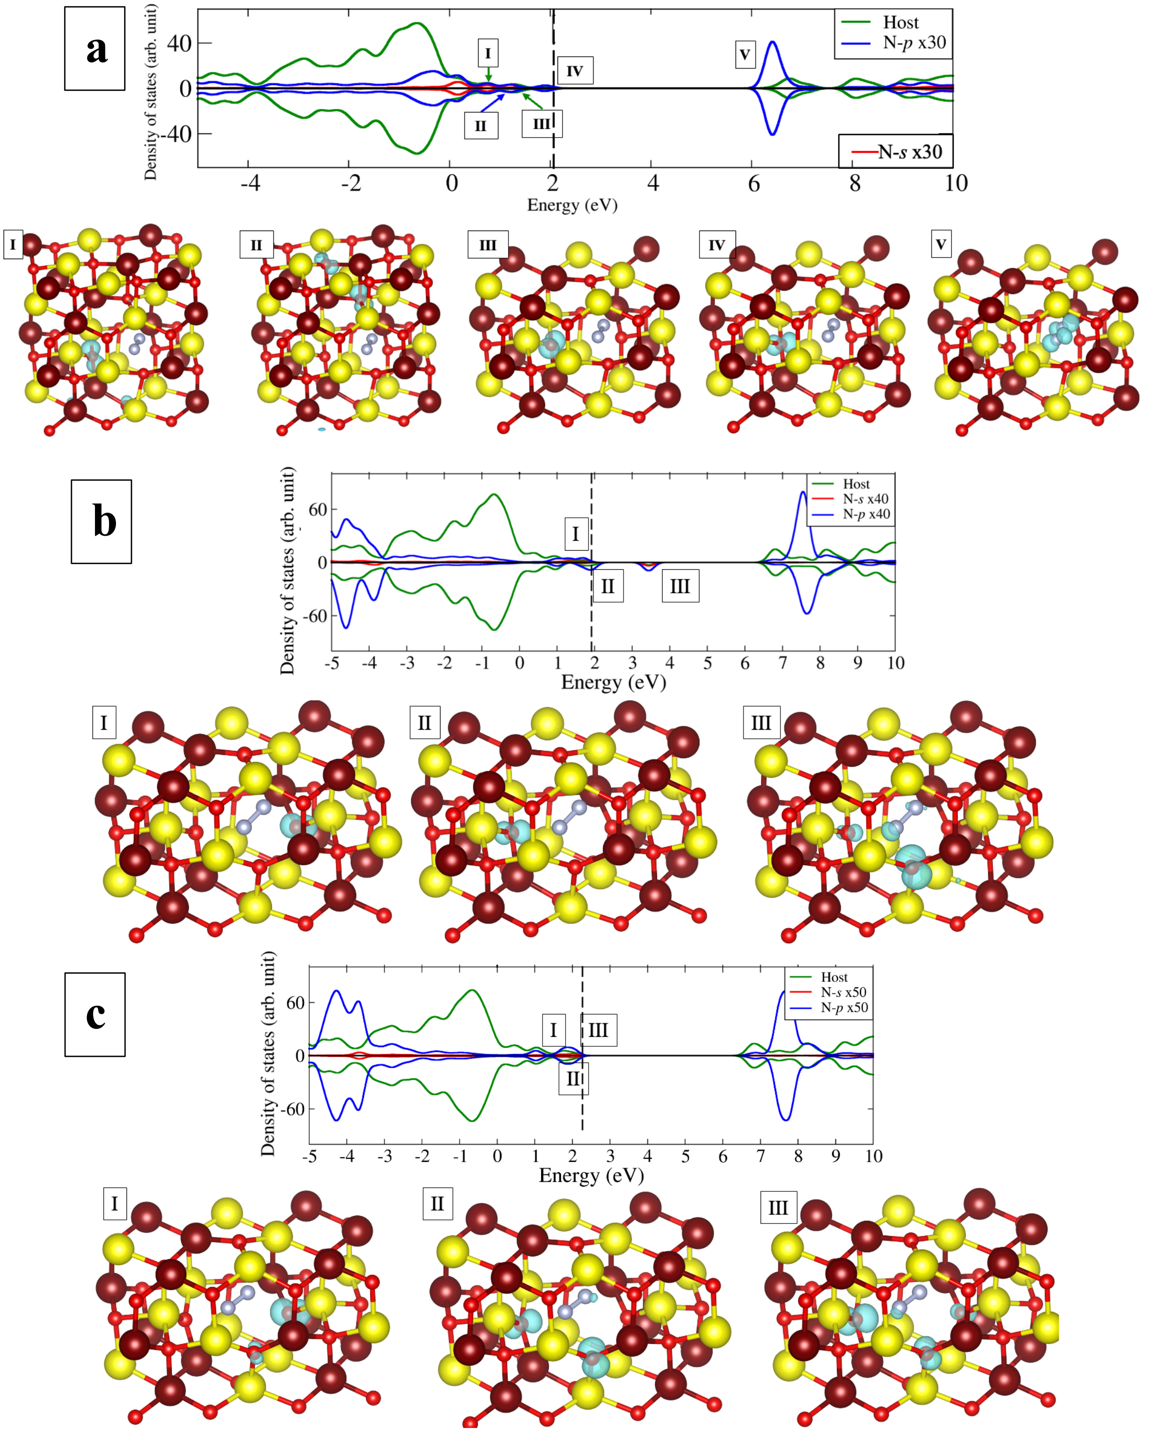


**Fig S9.** The partial density of state (PDOS) and the wave function localization of $(N_2)_{Ga}$ with (a) -1, (b) -2 and (c) -3 charge states, respectively.
